# Supplementary material for: Formulating Camera-Adaptive Color Constancy as a Few-shot Meta-Learning Problem
Source: arXiv:1811.11788 source file (2019-04-03)
Supplement: Supplementary file 1 [file supplementary_for_CVPR.tex]

\documentclass[10pt,twocolumn,letterpaper]{article}

\usepackage{cvpr}
\usepackage{times}
\usepackage{epsfig}
\usepackage{graphicx}
\usepackage{amsmath}
\usepackage{amssymb}
\usepackage{subfigure}
\usepackage{gensymb}

% Include other packages here, before hyperref.

% If you comment hyperref and then uncomment it, you should delete
% egpaper.aux before re-running latex.  (Or just hit 'q' on the first latex
% run, let it finish, and you should be clear).
\usepackage[breaklinks=true,bookmarks=false]{hyperref}

%\cvprfinalcopy % *** Uncomment this line for the final submission

 % *** Enter the CVPR Paper ID here

% Pages are numbered in submission mode, and unnumbered in camera-ready
\ifcvprfinal\pagestyle{empty}\fi
\begin{document}

%%%%%%%%% TITLE
\title{Meta-Learning for Few-shot Camera-Adaptive Color Constancy - Supplementary Material}

\author{First Author\\
Institution1\\
Institution1 address\\
{\tt\small firstauthor@i1.org}
\and
Second Author\\
Institution2\\
First line of institution2 address\\
{\tt\small secondauthor@i2.org}
}

\maketitle

\section{Task definition using color temperature histograms}

\noindent In our paper, a task is defined as a collection of images from a specific camera and from a specific bin of the CCT histogram.  We provide additional examples of CCT histograms and their corresponding clustering of ground-truth (GT) illuminant corrections in RGB space. Results for the $M\!=\!3$ bins case, for two cameras (Canon 600D and Nikon D40 from the NUS-9 dataset~\cite{cheng2014illuminant}) are shown in Fig.~\ref{fig:supp:CCT}. For the Canon 600D, Fig.~\ref{fig:supp:CCT:Canon600D_hist} shows an acceptable number of images in each bin for defining a task and~\ref{fig:supp:CCT:Canon600D_GT} exhibits the related ground-truth illuminant clustering for $M\!=\!3$. For the Nikon D40, a critical issue is that when using $M\!=\!3$ histogram bins, there are not enough images ($<10\!=\!K$) available in the first bin as shown in~\ref{fig:supp:CCT:D40_hist}. In Fig.~\ref{fig:supp:CCT:D40_GT} it can be observed that the ground-truth illuminants in bins two and three retain reasonable cluster separability, suggesting that more image data would help to make increased histogram granularity feasible. These results motivate the choice of $M\!=\!2$, as shown in Figure $4$ of the main paper, providing distinctive tasks with sufficient number of images in each bin of the CCT histogram.

% However, Fig.~\ref{fig:supp:CCT:Canon600D_GT} exhibits ground-truth illuminants in bins two and three that are not well separated (\emph{ie.}, the green and red glyphs exhibit overlap). Therefore, these overlapping tasks may be less distinctive than the $M\!=\!2$ bin setting.

% Also, as shown in Fig.~\ref{fig:supp:CCT:D40_GT}, the bins lack distinctive clusters (\emph{ie.}, the blue glyphs are not well separated from the red ones).

\begin{figure}[!t]
\begin{center}
\subfigure[Canon 600D histogram]{
    \label{fig:supp:CCT:Canon600D_hist}
    \includegraphics[width=0.22\linewidth]{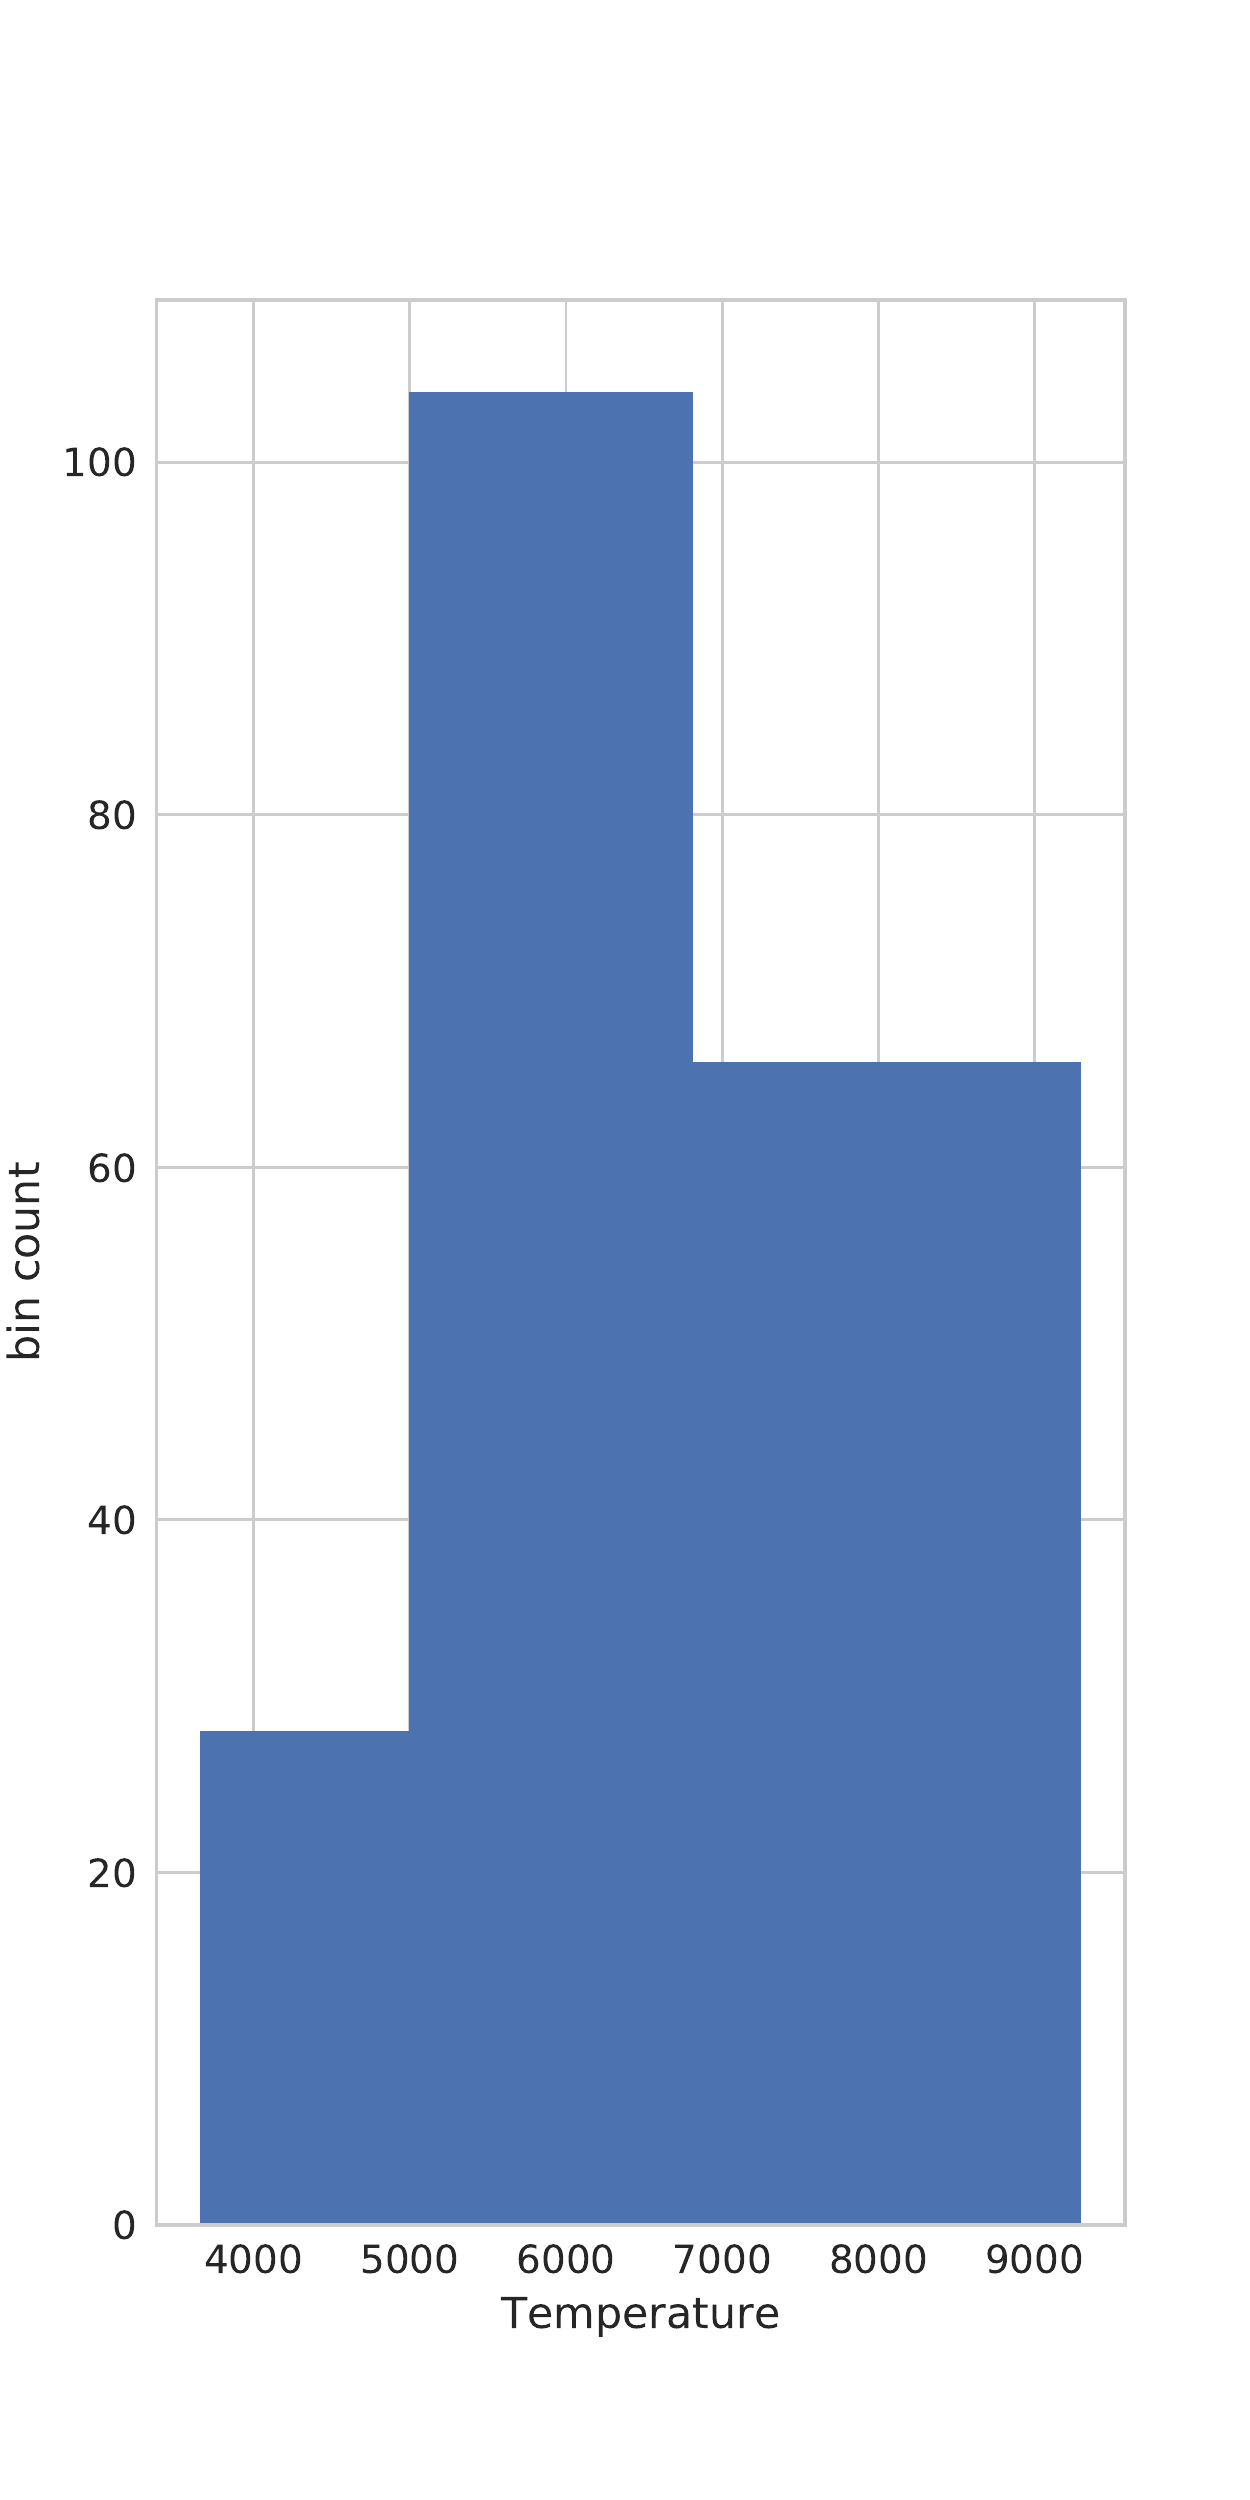}
    }
    \subfigure[Canon 600D GT illuminants in RGB space]{
    \label{fig:supp:CCT:Canon600D_GT}
    \includegraphics[width=0.70\linewidth]{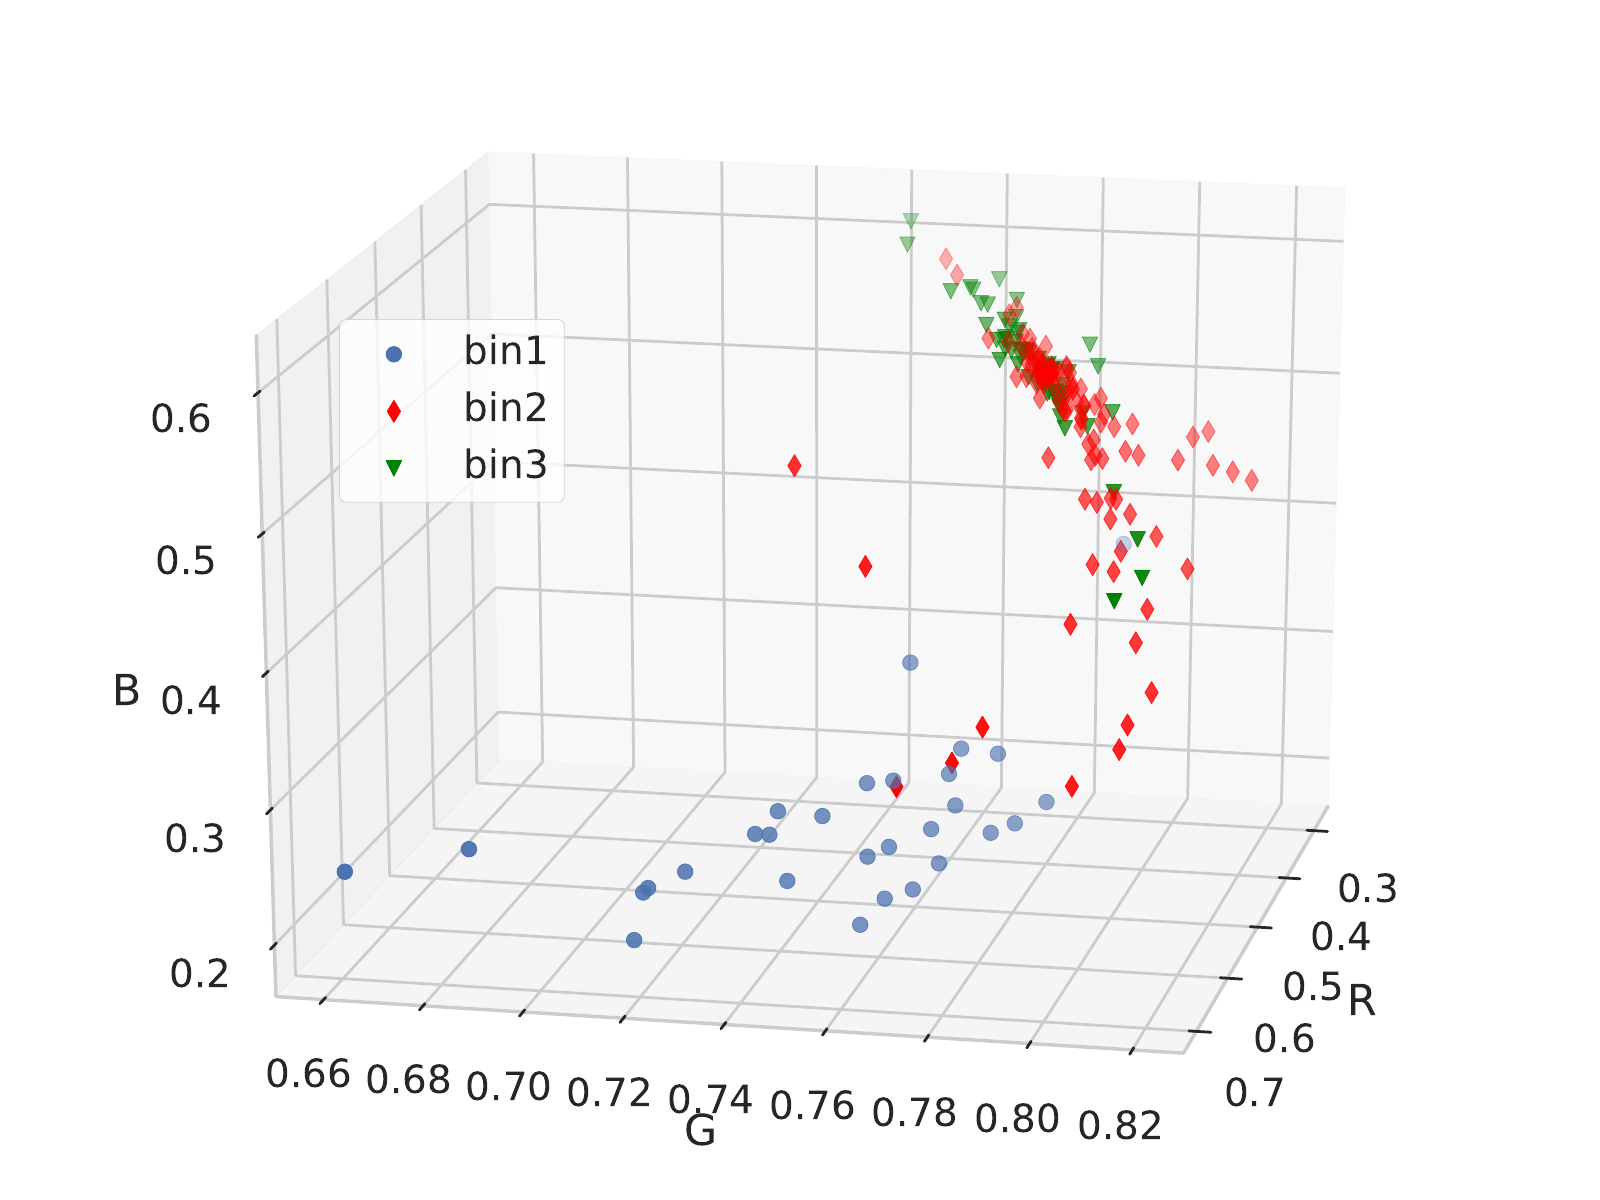}
    }
    \subfigure[Nikon D40 histogram]{
    \label{fig:supp:CCT:D40_hist}
    \includegraphics[width=0.22\linewidth]{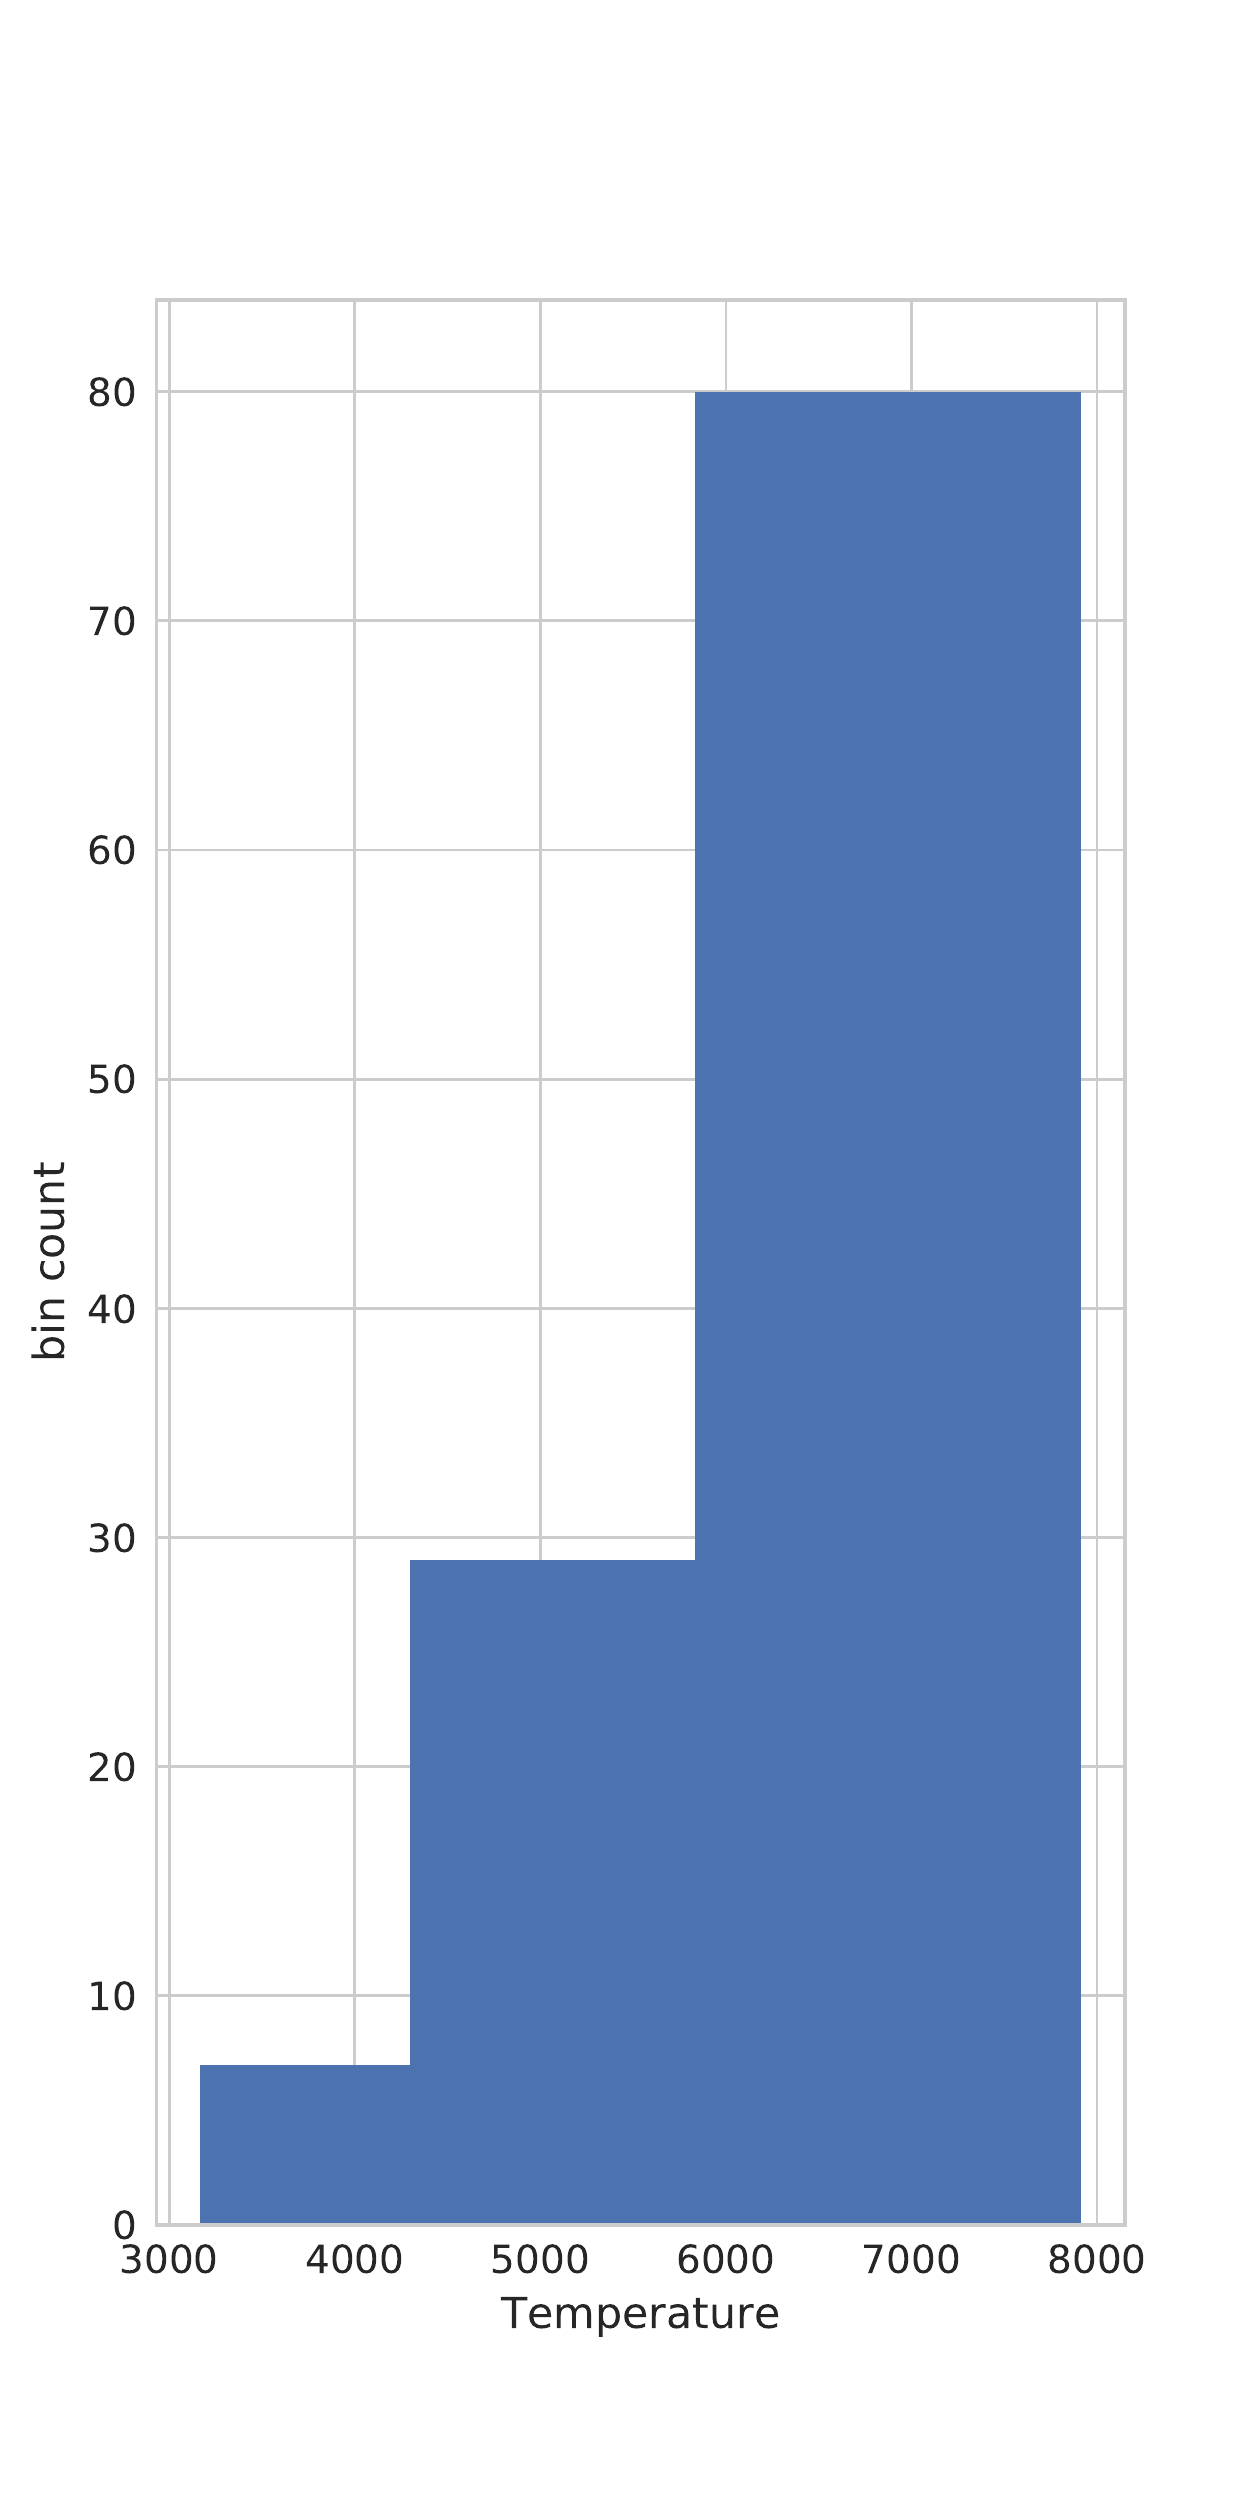}
    }
    \subfigure[Nikon D40 GT illuminants in RGB space]{
    \label{fig:supp:CCT:D40_GT}
    \includegraphics[width=0.70\linewidth]{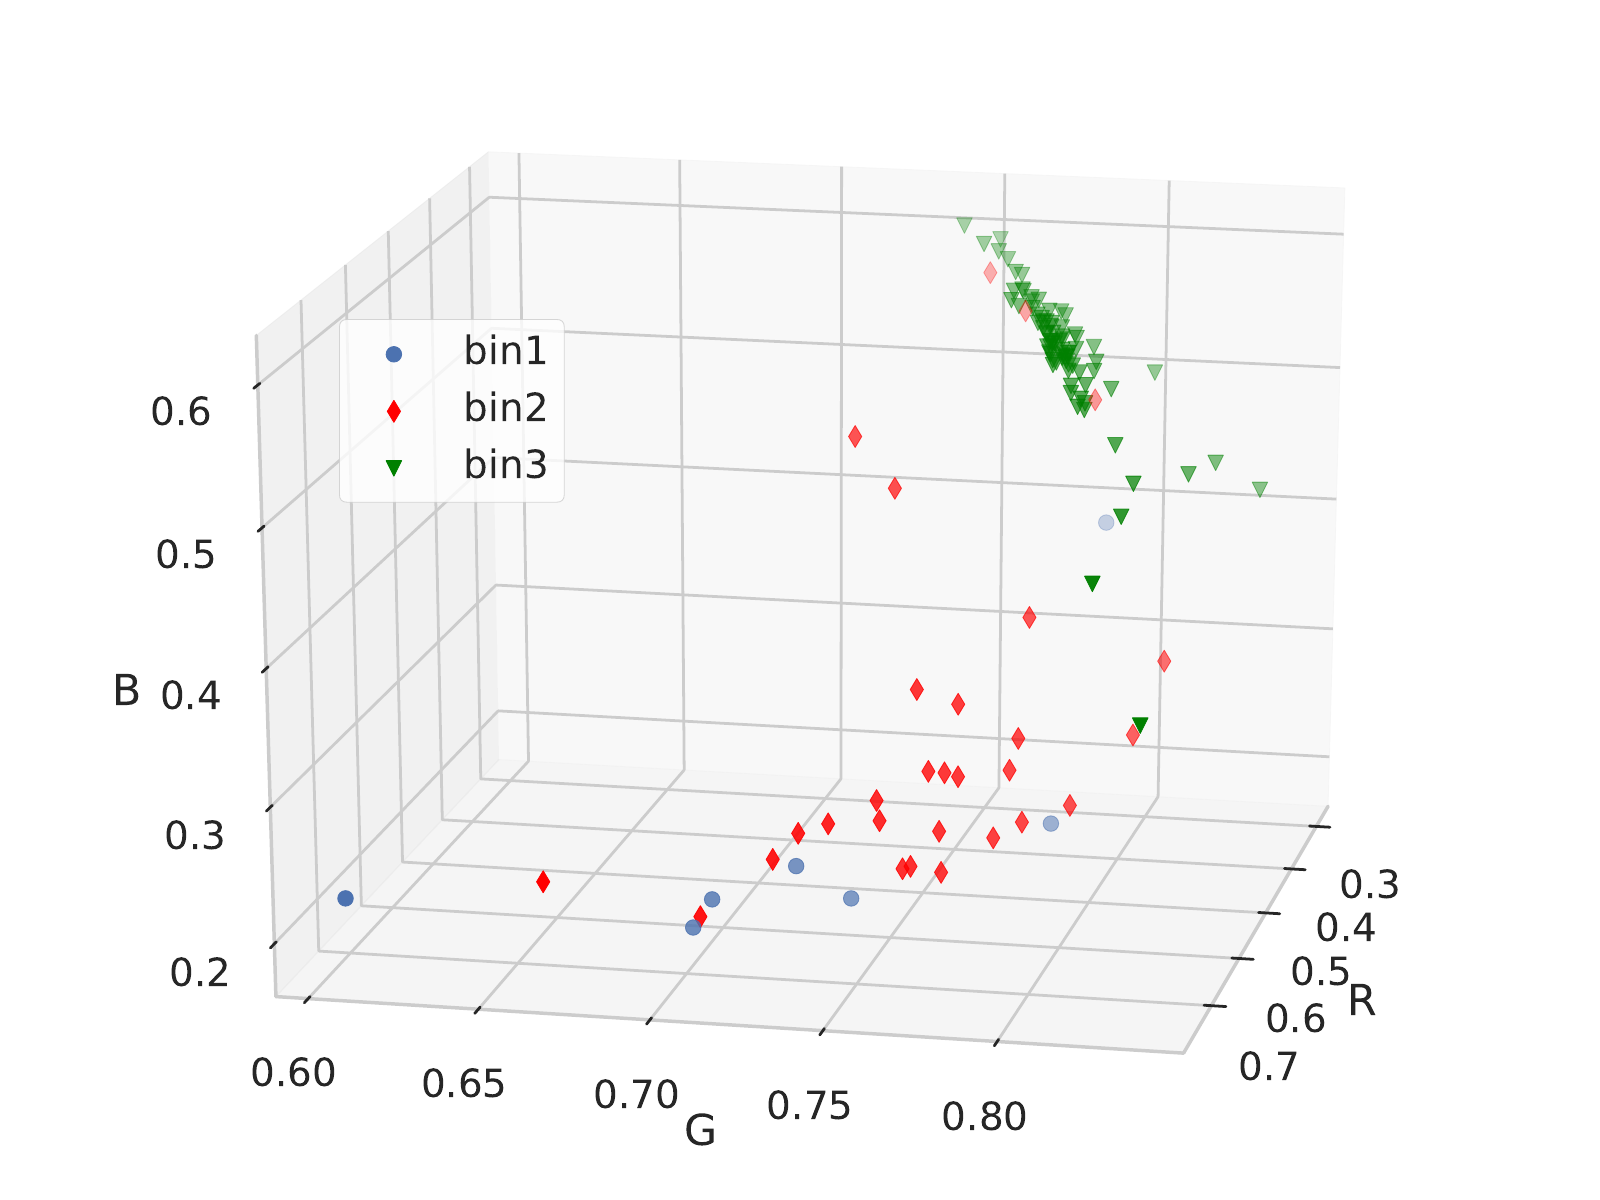}
    }
 \end{center}
\caption{CCT histograms $H_s$, 3 bin example.}
\label{fig:supp:CCT}
\end{figure}

\section{Base-learner architecture details}

\noindent Figure \ref{fig:supp:archi} shows the base-learner network architecture considered in our work. As described in the manuscript, the base architecture is composed of four convolutional layers (all sized $3\times3\times64$), an average pooling layer and two fully connected layers (sizes $64\times64$, $64\times3$) all with ReLU activations, except for the last layer.

\begin{figure}[t]
\centering
\includegraphics[width=1\linewidth]{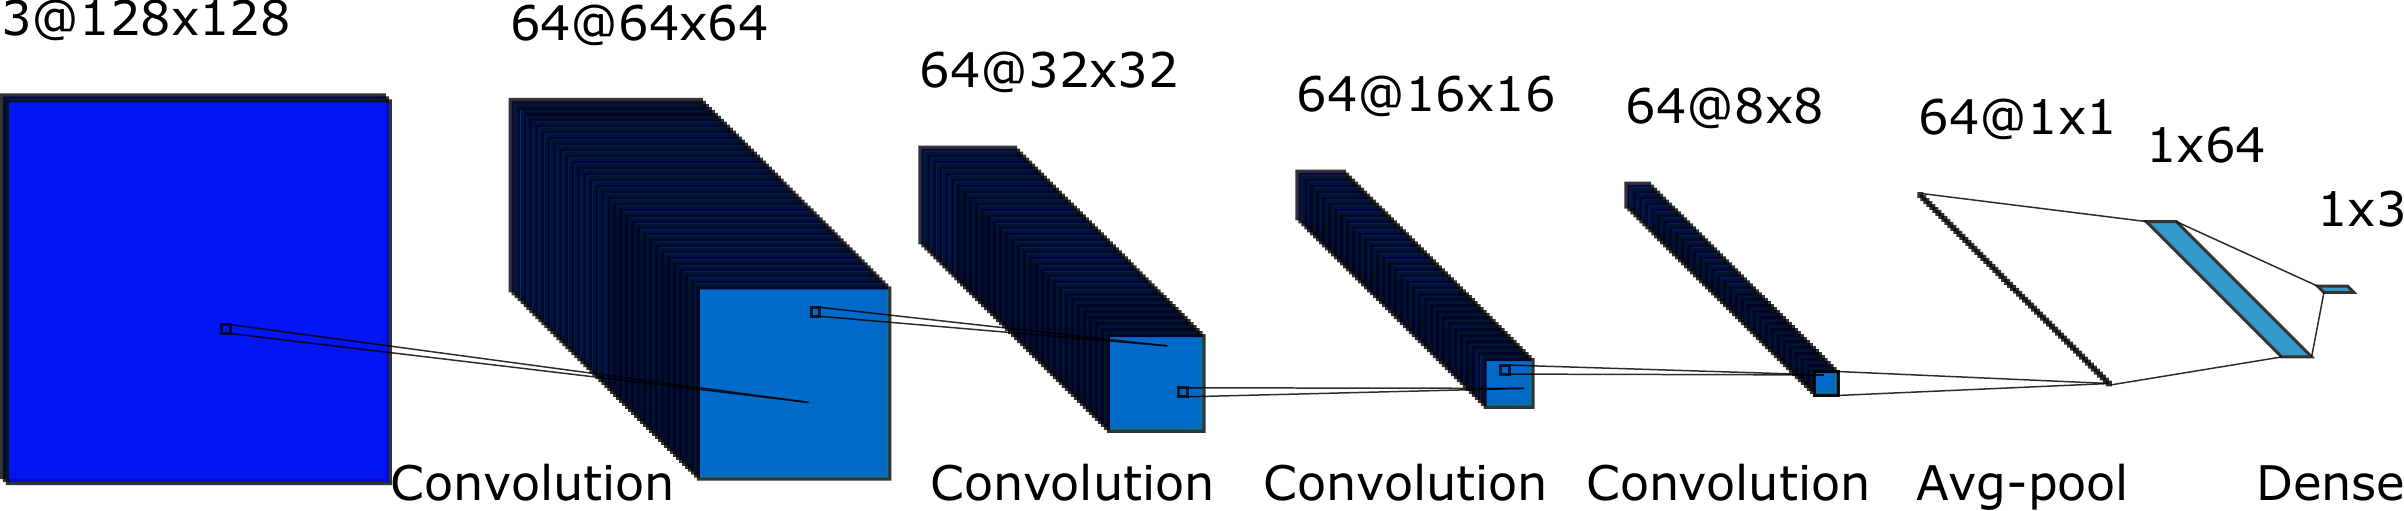}
\caption{Illustration of the considered network architecture.}
\label{fig:supp:archi}
\end{figure}

\section{Funt HDR data set}

\subsection{Image selection per scene}

We make use of the HDR image dataset captured by Funt and Shi~\cite{funt2010rehabilitation} and consider $95$ scenes for which ground-truth illuminants are available. The dataset contains subsets of (up to) $18$ images per scene, captured over short time frames (${\sim} 5$fps). During capture, the camera was able to auto-adjust shutter speed and aperture settings between frames~\cite{funt2010rehabilitation}. In other words, the $f$-stop setting was not fixed. We choose a representative image per scene by selecting a single exposure, shutter speed and aperture configuration and in practice we find the scene image with aperture $f$-stop nearest to $f/8$ in an attempt to balance between reasonable depth of field, retaining sharp objects in frame and also the amount of light admitted.    

%and discard $10$ scenes where all scene images contain the MCC. The Funt HDR dataset contributes $95$ distinct image samples to our accumulated total.

\subsection{Macbeth Color Checker}

In each scene, $4$ Macbeth Color Checkers (MCC) are present in positions such that the illumination incident is expected to represent overall scene illumination. To realise our (unique) dominant scene illuminant assumption, we compute the \emph{median GT illuminant} per scene to approximate a dominant illumination. In Figure \ref{fig:supp:FUNT_std} we investigate the validity of this approach. For each scene, we compute angular error between the \emph{median GT illuminant} and each of the $4$ distinct GT scene illuminants, provided by each MCC. Figure \ref{fig:supp:boxplotsfunt} shows per-scene boxplots of the computed angular errors. While we observe that most median errors are smaller than $2$ degrees, several images have very large angular differences between MCCs. This suggests that our single illuminant approximation may not be suitable for these images, explaining our relatively poorer performance on the Funt HDR dataset.

In Figure \ref{fig:supp:histfunt}, we show a histogram computing the minimum distance between (any) scene MCC illuminant and the \emph{median GT illuminant} (used in our paper as ground-truth). We observe that the large majority have a distance smaller than $1$ degree, suggesting that our approximation is very similar to an approach of choosing a single MCC as GT, under the single illuminant approximation.

\begin{figure}[!h]
\centering
\subfigure[Boxplot of the angular errors between our considered median GT and the GT illuminant of each MCC.]{
    \label{fig:supp:boxplotsfunt}
    \includegraphics[width=1\linewidth]{images/supp/FUNT_scene.pdf}
    }
    \subfigure[Histogram of the minimum angular error between each MCC and the median GT.]{
    \label{fig:supp:histfunt}
    \includegraphics[width=0.5\linewidth]{images/supp/FUNT_histscene.pdf}
    }
\caption{Intra-scene MCC ground-truth variability for considered FUNT HDR images~\cite{funt2010rehabilitation}.}
\label{fig:supp:FUNT_std}
\end{figure}

\section{Interpretation of NUS camera results}

The NUS-8 camera dataset~\cite{cheng2014illuminant} is comprised of subsets of ${\sim}210$ images representing largely similar scenes and illuminants captured by different cameras. Due to the scene and illumination invariance, differences in GT illuminant distributions can therefore be associated with differences in Camera Spectral Sensitivity (CSS). In Fig.~\ref{fig:supp:med_gain} we plot the \emph{median GT illuminant} correction in RGB space per camera for 8 NUS subsets and reproduce our NUS per camera accuracy results from the main manuscript, where we compared our approach with that of the baseline. 

By inspecting Fig.~\ref{fig:supp:med_gain:per_camera_GT}, it may be seen that the `Fujifilm' and `Olympus' cameras have distinct and relatively distant median GT in RGB space compared with the other cameras in the NUS dataset. This correlates well with the results we obtain using the baseline fine-tuning method, where the na\"ive fine-tuning of these two cameras results in weak median angular-error performance.  This is demonstrated in Fig.~\ref{fig:supp:med_gain:per_camera_results}, where larger errors for these cameras are observed for the baseline approach visualized in a blue color. On the contrary, our Meta-AWB approach is able to quickly adapt to large differences in camera sensor and yields consistent performance across all cameras investigated, demonstrated by consistently lower error, visualized in green.

It should be noted that the Nikon D40 camera GT is not plotted in Fig. \ref{fig:supp:med_gain:per_camera_GT}. Acquired later, this image set has substantially fewer images and no direct scene-to-scene correspondence, making a median GT comparison to the rest of the cameras less meaningful. The lack of scene correspondence may partially explain the weak baseline na\"ive fine-tuning results also observed for this camera.

\begin{figure}[t]
\centering
\subfigure[Median ground-truth RGB correction for NUS-8 cameras.]{
    \label{fig:supp:med_gain:per_camera_GT}
    \includegraphics[width=0.7\linewidth]{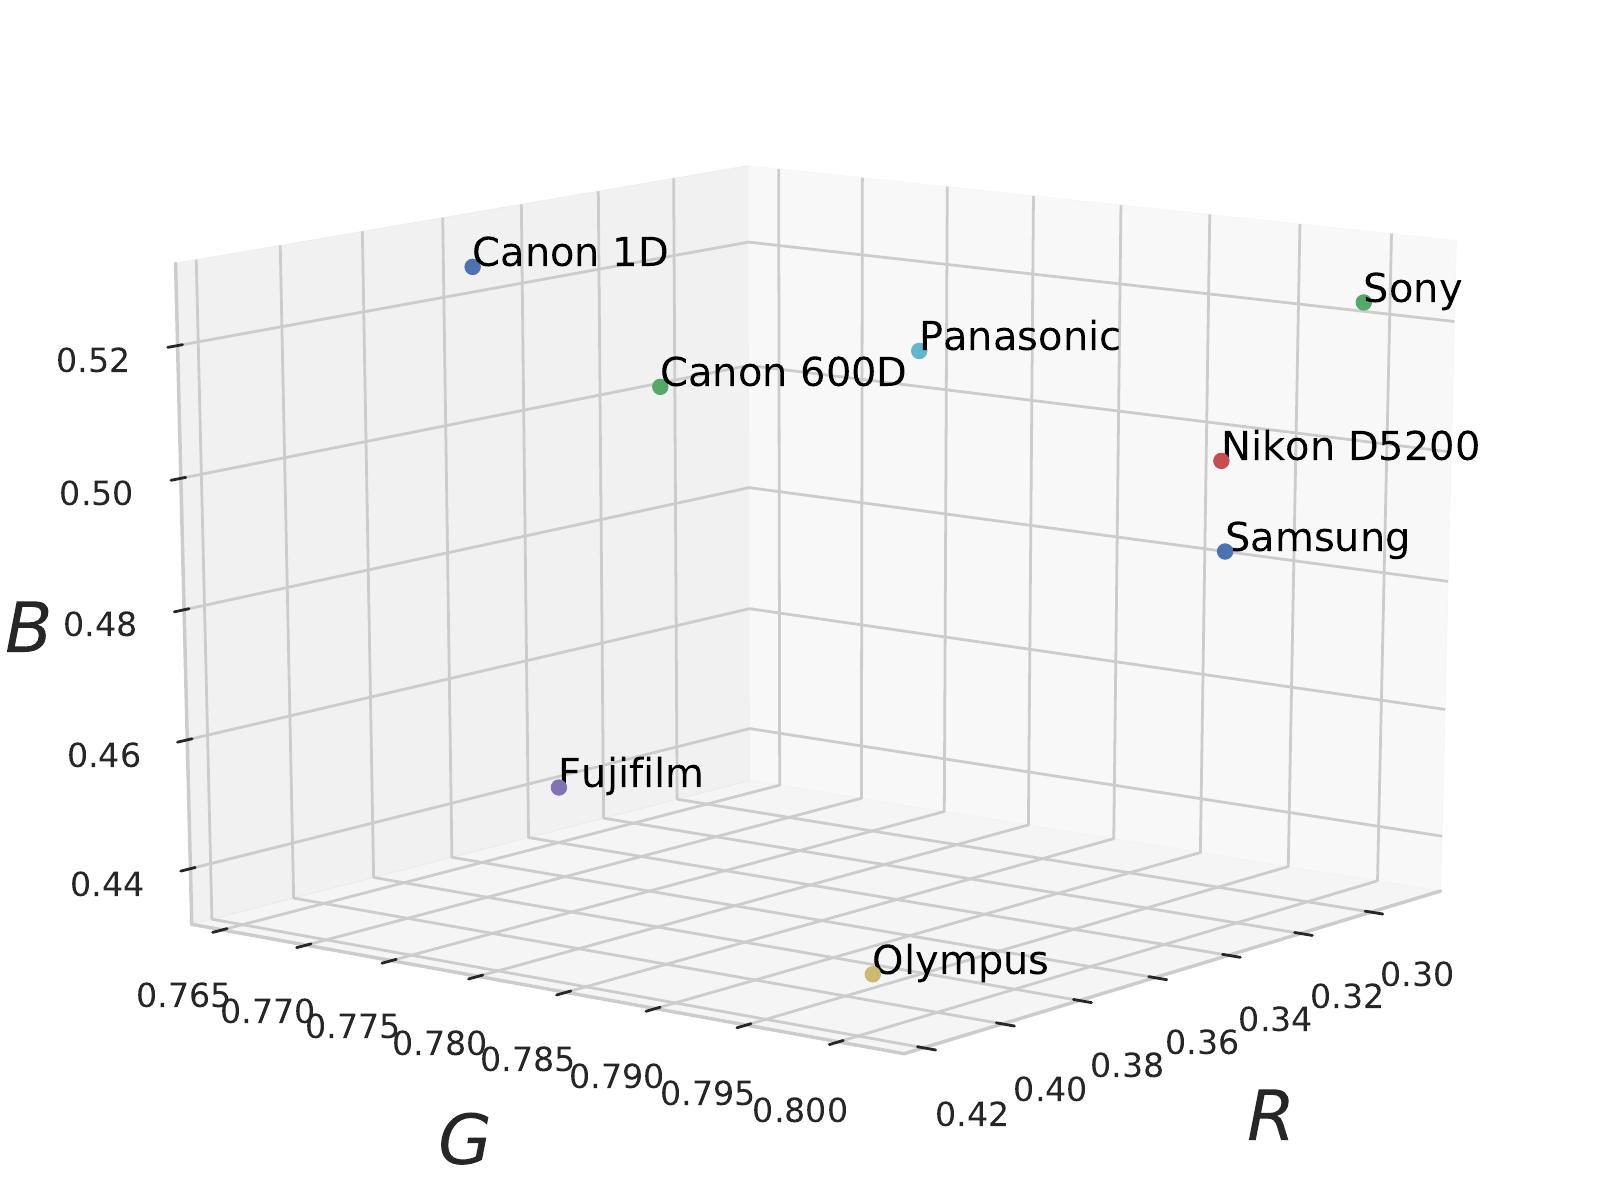}
    }
    \subfigure[Median angular error for each NUS camera, as shown in the main paper.]{
    \label{fig:supp:med_gain:per_camera_results}
    \includegraphics[width=1\linewidth]{images/sec4/NUSbar.pdf}
    }
\caption{Results on NUS-9 cameras and median GT RGB corrections.}
\label{fig:supp:med_gain}
\end{figure}

\section{Qualitative results}

In Figures~\ref{fig:supp:results1:log}-\ref{fig:supp:results6:log} we provide additional qualitative results in the form of images from the Gehler-Shi dataset~\cite{gehler2008bayesian,shi2000re}. For each image we show the input image produced by the camera and a white-balanced image corrected using the ground-truth illumination. We also show the output of our model (``Meta-AWB''), and that of the baseline fine-tuning approach reported in the paper. Color checker boards are visible in the images, however the relevant areas are masked prior to inference. Images are shown in sRGB space and clipped at the $97.5$ percentile. 

In similar fashion to~\cite{barron2015convolutional}, we adopt the strategy of sorting the $568$ images in the dataset by the combined mean angular-error of the evaluated methods. We present images of increasing average difficulty however images to report were selected by instead ordering from \emph{``hard''} to \emph{``easy''} and sampling with a logarithmic spacing, providing more samples that proved challenging on average.    

% We order the images from \emph{``easy''} to \emph{``hard''} and uniformly sample images $1,100,\ldots,500$.

%%%%%% LOGARITHMICALLY SAMPLED IMAGES %%%%%%

% LOGARITHMICALLY SAMPLING OF HARD --> EASY
% display_inds_log: 70 85 554 244 439 137 
% display_err_vec_maml:      9.111512  4.406820  5.908046 4.531664 1.242908 0.748512 
% display_err_vec_vanilla:  26.516517 24.026911 20.973234 5.763892 2.074942 0.526275

\begin{figure*}[!h]
\centering
    \subfigure[Input image]{
    \label{fig:supp:results1:log:subfig1}
    \includegraphics[width=0.45\linewidth]{images/supp/qual_results/log_sampling/95perc_qual/0137_input-fs8.png}
    }
    \subfigure[Ground-truth solution]{
    \label{fig:supp:results1:log:subfig2}
    \includegraphics[width=0.45\linewidth]{images/supp/qual_results/log_sampling/95perc_qual/0137_GT-fs8.png}
    }
    \subfigure[Meta-AWB, err = $0.74\degree$]{
    \label{fig:supp:results1:log:subfig3}
    \includegraphics[width=0.45\linewidth]{images/supp/qual_results/log_sampling/95perc_qual/0137_maml-fs8.png}
    }
    \subfigure[Baseline fine-tuning, err = $0.52\degree$]{
    \label{fig:supp:results1:log:subfig4}
    \includegraphics[width=0.45\linewidth]{images/supp/qual_results/log_sampling/95perc_qual/0137_vanilla-fs8.png}
    }
\caption{For each scene we present the input image produced by the camera alongside the ground-truth white-balanced image. Images are shown in sRGB space and normalized to the $97.5$th percentile. For both our `Meta-AWB' approach and the baseline algorithm we show the white-balanced image, as well as the angular-error of the estimated illumination in degrees, with respect to the ground-truth.}
\label{fig:supp:results1:log}
\end{figure*}

\begin{figure*}[!h]
\centering
    \subfigure[Input image]{
    \label{fig:supp:results2:log:subfig1}
    \includegraphics[width=0.45\linewidth]{images/supp/qual_results/log_sampling/95perc_qual/0439_input-fs8.png}
    }
    \subfigure[Ground-truth solution]{
    \label{fig:supp:results2:log:subfig2}
    \includegraphics[width=0.45\linewidth]{images/supp/qual_results/log_sampling/95perc_qual/0439_GT-fs8.png}
    }
    \subfigure[Meta-AWB, err = $1.24\degree$]{
    \label{fig:supp:results2:log:subfig3}
    \includegraphics[width=0.45\linewidth]{images/supp/qual_results/log_sampling/95perc_qual/0439_maml-fs8.png}
    }
    \subfigure[Baseline fine-tuning, err = $2.07\degree$]{
    \label{fig:supp:results2:log:subfig4}
    \includegraphics[width=0.45\linewidth]{images/supp/qual_results/log_sampling/95perc_qual/0439_vanilla-fs8.png}
    }
\caption{Additional results in the same format as Figure~\ref{fig:supp:results1:log}}
\label{fig:supp:results2:log}
\end{figure*}

\begin{figure*}[!h]
\centering
    \subfigure[Input image]{
    \label{fig:supp:results3:log:subfig1}
    \includegraphics[width=0.45\linewidth]{images/supp/qual_results/log_sampling/95perc_qual/0244_input-fs8.png}
    }
    \subfigure[Ground-truth solution]{
    \label{fig:supp:results3:log:subfig2}
    \includegraphics[width=0.45\linewidth]{images/supp/qual_results/log_sampling/95perc_qual/0244_GT-fs8.png}
    }
    \subfigure[Meta-AWB, err = $4.53\degree$]{
    \label{fig:supp:results3:log:subfig3}
    \includegraphics[width=0.45\linewidth]{images/supp/qual_results/log_sampling/95perc_qual/0244_maml-fs8.png}
    }
    \subfigure[Baseline fine-tuning, err = $5.76\degree$]{
    \label{fig:supp:results3:log:subfig4}
    \includegraphics[width=0.45\linewidth]{images/supp/qual_results/log_sampling/95perc_qual/0244_vanilla-fs8.png}
    }
\caption{Additional results in the same format as Figure~\ref{fig:supp:results1:log}}
\label{fig:supp:results3:log}
\end{figure*}

\begin{figure*}[!h]
\centering
    \subfigure[Input image]{
    \label{fig:supp:results4:log:subfig1}
    \includegraphics[width=0.45\linewidth]{images/supp/qual_results/log_sampling/95perc_qual/0554_input-fs8.png}
    }
    \subfigure[Ground-truth solution]{
    \label{fig:supp:results4:log:subfig2}
    \includegraphics[width=0.45\linewidth]{images/supp/qual_results/log_sampling/95perc_qual/0554_GT-fs8.png}
    }
    \subfigure[Meta-AWB, err = $5.90\degree$]{
    \label{fig:supp:results4:log:subfig3}
    \includegraphics[width=0.45\linewidth]{images/supp/qual_results/log_sampling/95perc_qual/0554_maml-fs8.png}
    }
    \subfigure[Baseline fine-tuning, err = $20.97\degree$]{
    \label{fig:supp:results4:log:subfig4}
    \includegraphics[width=0.45\linewidth]{images/supp/qual_results/log_sampling/95perc_qual/0554_vanilla-fs8.png}
    }
\caption{Additional results in the same format as Figure~\ref{fig:supp:results1:log}}
\label{fig:supp:results4:log}
\end{figure*}

\begin{figure*}[!h]
\centering
    \subfigure[Input image]{
    \label{fig:supp:results5:log:subfig1}
    \includegraphics[width=0.45\linewidth]{images/supp/qual_results/log_sampling/95perc_qual/0085_input-fs8.png}
    }
    \subfigure[Ground-truth solution]{
    \label{fig:supp:results5:log:subfig2}
    \includegraphics[width=0.45\linewidth]{images/supp/qual_results/log_sampling/95perc_qual/0085_GT-fs8.png}
    }
    \subfigure[Meta-AWB, err = $4.40\degree$]{
    \label{fig:supp:results5:log:subfig3}
    \includegraphics[width=0.45\linewidth]{images/supp/qual_results/log_sampling/95perc_qual/0085_maml-fs8.png}
    }
    \subfigure[Baseline fine-tuning, err = $24.02\degree$]{
    \label{fig:supp:results5:log:subfig4}
    \includegraphics[width=0.45\linewidth]{images/supp/qual_results/log_sampling/95perc_qual/0085_vanilla-fs8.png}
    }
\caption{Additional results in the same format as Figure~\ref{fig:supp:results1:log}}
\label{fig:supp:results5:log}
\end{figure*}

\begin{figure*}[!h]
\centering
    \subfigure[Input image]{
    \label{fig:supp:results6:log:subfig1}
    \includegraphics[width=0.45\linewidth]{images/supp/qual_results/log_sampling/95perc_qual/0070_input-fs8.png}
    }
    \subfigure[Ground-truth solution]{
    \label{fig:supp:results6:log:subfig2}
    \includegraphics[width=0.45\linewidth]{images/supp/qual_results/log_sampling/95perc_qual/0070_GT-fs8.png}
    }
    \subfigure[Meta-AWB, err = $9.11\degree$]{
    \label{fig:supp:results6:log:subfig3}
    \includegraphics[width=0.45\linewidth]{images/supp/qual_results/log_sampling/95perc_qual/0070_maml-fs8.png}
    }
    \subfigure[Baseline fine-tuning, err = $26.51\degree$]{
    \label{fig:supp:results6:log:subfig4}
    \includegraphics[width=0.45\linewidth]{images/supp/qual_results/log_sampling/95perc_qual/0070_vanilla-fs8.png}
    }
\caption{Additional results in the same format as Figure~\ref{fig:supp:results1:log}}
\label{fig:supp:results6:log}
\end{figure*}

{\small
\bibliographystyle{ieee}
\bibliography{egbib}
}

\end{document}
